# Supplementary material for: Localized Energy States Induced by Atomic-Level Interfacial Broadening in Heterostructures
Source: arXiv:2203.14419 ancillary file (2022-03-28)
Supplement: Supplementary file 1 [file SLs_Interface_Abs_SM.pdf]

**Supplementary Material:**

# Localized Energy States Induced by Atomic-Level Interfacial Broadening in Heterostructures

*Anis Attiaoui,[1] Gabriel Fettu,[1] Samik Mukherjee,[1] Matthias Bauer,[2] and Oussama Moutanabbir[1]*

*[1]Department of Engineering Physics, École Polytechnique de Montréal, C. P. 6079, Succ. Centre-Ville, Montréal, Québec H3C 3A7, Canada*
*[2] Applied Materials Inc., 974 E. Arques Avenue, Sunnyvale, CA 94085, USA*

## Contents

S1. 14-band $k{\cdot}p$ Optical Absorption .......... 2
S2. Structural characterization of all SLs .......... 10
S3. Atom Probe Tomography (APT) Characterization .......... 10
S4. Characterization of lattice Strain .......... 12
S5. Atomic Force Microscopy (AFM) Characterization .......... 13
S6. Spectroscopic Ellipsometry (SE) .......... 14
S7. Fitting second derivative lineshapes .......... 16
References .......... 19

## S1. 14-band *k·p* Optical Absorption

The band structures of the Si/SiGe superlattices were calculated using the 14-band *k·p* model together with the envelope function approximation (EFA). [1] In systems composed of semiconductors such as GaAs or Ge, using an 8-band k·p model is enough to model the optical properties close to the band gap, because the $\Gamma_2^-$ CB (s-type) is the lowest conduction band. In Si or Si-rich SiGe, the lowest conduction band has the $\Gamma_4^- /(\Gamma_8^- + \Gamma_6^-)$ symmetry (p-type), and the $\Gamma_2^-$ CB is not very far in energy, hence the necessity of a 14-band *k·p* model. The strain implementation is based on the Bir-Pikus formalism. [2] In k·p models with a relatively low number of bands, such as the 8 band and 14 band models, the effect of remote bands on the conduction band are considered by specific parameters denoted by $\gamma_{Cj}$ . These parameters can have great impacts on the accuracy of the calculated band structures. In bulk Si and Ge, since electrons do not fill the Γ conduction band states, there are no experimental cyclotron resonance data available for the $\gamma_{Cj}$ parameters. [1] To estimate these parameters for Si and SiGe, the 14-band *k·p* model was fitted to a 30-band model, which includes the exact remote band states effect. Another possibility would have been to directly use the 30-band model to evaluate the optical absorption in superlattices. However, this leads to much higher computation time, and the use of the 30-band model for superlattices has several well documented issues. [3]

### Luttinger-like $\gamma_{Cj}$ parameters

The $\gamma_{Cj}$ remote band parameters of the 14-band *k·p* model for bulk Si, Ge and SiGe alloys were fitted to a 30-band model [4] by using a quasi-Newton method optimization algorithm. This optimization is based on a least-squares error between the energy levels of the 14-band model and the same levels in the 30-band model, along the [001], [111] and [110] directions. The 14-band *k·p* model is limited to a region in the Brillouin zone relatively close to the Γ point, contrary to the 30-band model which is valid in the full Brillouin zone. Therefore, a maximum wave vector norm of 2/nm was selected for the fitting between the two methods.

The fitting procedure is shown in Figure S1 (a) for Si. Due to the lack of experimental values for $\gamma_{Cj}$ parameters, the remote band effects on the p-type conduction band were not included. [1] In our work, this assumption is used as an initial guess for the optimization algorithm.

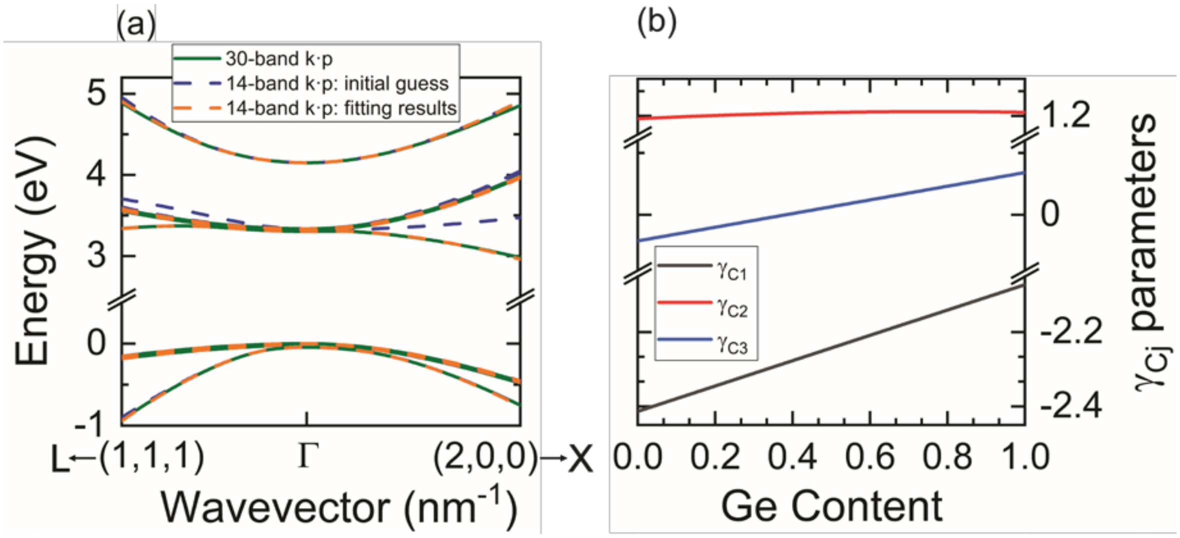


Figure S1: (a) Band structure of Si evaluated with a 14-band k·p model fitted to a 30-band k·p model, which is also shown. The parameters used as variable for the fit are the Luttinger and $\gamma_{Cj}$ parameters. (b) The $\gamma_{Cj}$ parameters obtained from the fitting procedure.

After completion of the fit, the conduction bands obtained with the 14-band *k·p* model match much more closely the results with the 30-band *k·p* model. The optimization is repeated for various SiGe compositions that span the full range of alloys, to obtain the $\gamma_{Cj}$ parametrization shown in Figure S1 (b). The polynomial fit equations for $\mathrm{Si_{1-x}Ge_x}$ alloys are presented below.

$$\gamma_{C1} = -2.072x - 2.413(1-x)$$

$$\gamma_{C2} = 1.2096x + 1.192(1-x) + 0.0328\,x(1-x)$$

$$\gamma_{C3} = 0.1137x - 0.0704(1-x)$$

## SiGe 14-band *k·p* parametrization

The $\mathrm{Si_{1-x}Ge_x}$ material parameters used in the *k·p* calculation are summarized in Table S1. The appropriate bowing parameters for both SiGe and Ge were used when available. In this work, the bowing parameter $b_{\mathrm{Si_{1-x}Ge_x}}$ is used to account for the non-linear change of parameters from the linearly extrapolated Si and Ge values as

$$\Omega_{\mathrm{Si_{1-x}Ge_x}} = x\Omega_{\mathrm{Ge}} + (1-x)\Omega_{\mathrm{Si}} - x(1-x)b_{\mathrm{Si_{1-x}Ge_x}} \quad (1)$$

where $\Omega_{Ge}$ , $\Omega_{Si}$ and $\Omega_{Si_{1-x}Ge_x}$ are the given parameter values for the Ge, Si and $Si_{1-x}Ge_x$ semiconductors, respectively. The temperature dependence of the bandgap uses the Varshni relationship defined as

$$E_g^i(T) = E_g^i(0K) - \frac{\alpha_i}{T + \beta_i} \tag{2}$$

where $i = \Gamma, L$ or $X$ depends on which conduction band valley is considered. Finally, the temperature dependence of the lattice parameter of Si and Ge is defined through a 4-order polynomial based on the work of Reeber et *al*. [5]

$$a_0(T) = a_0(0K) + \sum_{i=1}^{4} k_i T^i \tag{3}$$

where the $k_i$ parameters are defined in Table S1 for both Si and Ge.

**Elimination of spurious solutions**

It is well known that band structure numerical evaluation of heterostructures obtained with a *k·p* framework is prone to the generation of unphysical "spurious" solutions. Different explanations, such as the incompleteness of the basis states used for the construction of the Hamiltonian, the experimental parameters used, or the chosen discretization scheme have been described extensively in literature. [6] These spurious solutions need to be identified and removed from the energy spectrum of the quantum well. To this end, the envelope-function spinor components of the states were analysed. It was found that the states in the middle of the band gap, which are clearly nonphysical, have very specific dominant spinor components. This made possible the creation of a criterion, labelled as X, to separate the real states from the non-physical ones, based on the value of 4 spinor components: $|\mathrm{c}\frac{1}{2}\rangle$, $|\mathrm{c}-\frac{1}{2}\rangle$, $|\mathrm{c}\frac{7}{2}\rangle$, $|\mathrm{c}-\frac{7}{2}\rangle$ (notation is the same as the one used in Ref. [7], for the 14-band *k·p* Hamiltonian basis spinors). At each wavenumber considered in the calculation, the criterion is then normalized by the maximum value of X among all the states.

$$X = \left(\left\langle \mathrm{c}\frac{1}{2}\middle|\mathrm{c}\frac{1}{2}\right\rangle + \left\langle \mathrm{c}-\frac{1}{2}\middle|\mathrm{c}-\frac{1}{2}\right\rangle\right) * \left(\left\langle \mathrm{c}\frac{7}{2}\middle|\mathrm{c}\frac{7}{2}\right\rangle + \left\langle \mathrm{c}-\frac{7}{2}\middle|\mathrm{c}-\frac{7}{2}\right\rangle\right); \quad X_{norm} = X/\max(X) \tag{4}$$

Table S1: The input parameters used in the 14-band $k\cdot p$ simulation

| Parameters | Silicon | Germanium | $Si_{1-x}Ge_x$ bowing |
|---|---|---|---|
| Lattice constant, $a_0$ (Å) at 0 K | 5.43[a] | 5.6522[a] | 0.027[b] |
| Temperature dependence of $a_0$, | | | |
| $k_1$ | -8.6332e-6[a] | 1.0330e-6[a] | |
| $k_2$ | 5.2699e-8[a] | 7.8398e-8[a] | |
| $k_3$ | -4.0261e-11[a] | -6.9653e-11[a] | |
| $k_4$ | 1.1759e-14[a] | 2.3033e-14[a] | |
| CB effective mass, $m_{c\Gamma}$ ($m_0$) | 0.241[c] | 0.0383[c] | 0.077135[c] |
| Band gaps, | | | |
| $E_0$ ($\Gamma$, eV) | 4.15[h] | 0.89[h] | |
| $E_0'$ ($\Gamma$, eV) | 3.302[h] | 2.923[h] | |
| $E_g$ (L, eV) | 2.01[p] | 0.785[d] | |
| $E_g$ ($\Delta$, eV) | 1.17[q] | 0.931[p] | 0.206[p] |
| Spin orbit coupling, | | | |
| $\Delta$ (meV) | 44[h] | 296[h] | 52[h] |
| $\Delta_C$ (meV) | 33[h] | 190[h] | |
| Varshni parameters, | | | |
| $\alpha(E_0, meV/K)$ | 536.7[e] | 684.2[e] | |
| $\beta(E_0, K)$ | 745.8[e] | 398[e] | |
| $\alpha(E_0', meV/K)$ | 350[m] | 360[l] | |
| $\beta\left(E_0', K\right)$ | 580[m] | 344[l] | |
| $\alpha_L(meV/K)$ | 536.7[e] | 456.1[e] | |
| $\beta_L(K)$ | 745.8[e] | 210[e] | |
| $\alpha_X(meV/K)$ | 702.1[e] | 477.4[e] | |
| $\beta_X(K)$ | 1108[e] | 235[e] | |
| Average valence band, $E_{v,avg}$ (eV) | -7.03[f] | -6.35[f] | |
| Elastic constant, $c_{11}$ (Gpa) | 167.5[g] | 131.5[g] | |
| Elastic constant, $c_{12}$ (GPa) | 65[g] | 49.4[g] | |
| Elastic constant, $c_{44}$ (GPa) | 80.1[g] | 68.4[g] | |
| Deformation potential constants,* | | | |
| $a_c^\Gamma$ (eV) | -5.1[k] | -9.5[k] | |
| $a_c^L$ (eV) | -0.66[n] | -1.54[n] | |
| $a_c^X$ (eV) | 3.3[o] | 2.55[n] | |
| $a_v$ (eV) | 2.46[f] | 1.24[f] | |
| $b$ (eV) | -2.10[i] | -2.86[j] | |
| $d$ (eV) | -4.85[i] | -5.28[j] | |
| Luttinger-like parameters,** | | | |
| $\gamma_1$ | 4.589 | 9.697 | 7.117 |
| $\gamma_2$ | 0.512 | 2.835 | 3.543 |
| $\gamma_3$ | 1.566 | 4.012 | 3.544 |
| $\gamma_{C1}$ | -2.413 | -2.072 | |
| $\gamma_{C2}$ | 1.192 | 1.2096 | -0.0328 |
| $\gamma_{C3}$ | -0.0704 | 0.1137 | |
| Coupling parameters | | | |
| $E_P(eV)$ | 20.25[h] | 19.14[h] | |
| $E_{PX}(eV)$ | 15.52[h] | 15.71[h] | |

*: The convention $a = a_c - a_v$ is used.
**: Parameters obtained from fitting procedure to a 30-band k·p model
[a]Reference [5].
[b]Reference [8]
[c]Reference [9].
[d]Reference [10].
[e]Reference [11].
[f]Reference [12].
[g]Reference [13].
[h]Reference [4].
[i]Reference [14].
[j]Reference [15].
[k]Reference [7].
[l]Reference [16].
[m]Reference [17].
[n]Reference [18].
[o]Reference [19].
[p]Reference [20].
[q]Reference [21].

We found that setting a simple threshold for $X_{norm}$ was enough to remove most of the spurious solutions. States with an $X_{norm}$ value superior to the threshold are defined as spurious, and states with an $X_{norm}$ value inferior to the threshold are defined as real. An optimal threshold of 0.75 was used for the calculations.

**Microscopic interface Hamiltonian**

Eight-band k.p formalism has been heavily used in literature to study the optical properties of short-period, strain-balanced and asymmetric SLs for group III-V and IV semiconductors. Foreman [22] proved rigorously that the IF potential has a short-range nature, which can be modelled by the $\delta$ function. Ivchencko et *al*. [23] deduced the IF Hamiltonian based on the theory of invariants, and only included the off-diagonal elements. Szmulovitch et *al*. [24] developed a modified 8×8 envelope-function approximation (EFA) formalism for III-V SL. With two adjustable parameters for the two possible interfaces, they found very good agreement between experiment and theory for the band gaps. In this work, the same formalism is extended to the 14-band k.p model for group IV SLs. Briefly, the interface asymmetry Hamiltonian is defined as

$$H_{IF} = \Theta a_0 [H_1^{BA}\delta(x+b) - H_2^{AB}\delta(x-b)] \quad (5)$$

where $\Theta$ is a mixing operator, introduced by Ivchenko et *al*. [23] that introduces coupling between the light-hole (LH) - heavy hole (HH) and HH-SO (spin orbit) states in the valence band and $a_0$ is the lattice parameter (here the parallel lattice constant of the SL). The delta functions represent the SL interfaces. For a SiGe/Si SL, there are two possible different interfaces- the Si-on-SiGe interface at $x = -b$ and the SiGe-on-Si interface at $x = b$. $H_1^{BA}$ and $H_2^{AB}$ are the strength of the interface potential, intrinsic to the internal structure of the SLs and are usually extracted experimentally by fitting the fundamental band gap to the thickness of the heterostructure, when

available. To use accurate values for the interface profiles, the APT measurements for the different SLs were exploited. A fit was applied to the data as described in S2, based on a sigmoid model as shown in Eq. (9). The values for the strength of the interface potential, represented by $H_1^{BA}$ and $H_2^{AB}$, were obtained by fitting the theoretical results to the ellipsometry measurements. Fixing $H_2^{AB}$ to 0 eV and using a value of 1.4 eV for $H_1^{BA}$ generated the most accurate theoretical results.

### Optical absorption coefficient

The theoretical value of the absorption coefficient $\alpha(\omega)$ was evaluated according to the Fermi Golden rule as indicated in the following equation [25]:

$$\alpha(\omega) = \frac{\pi e^2}{n_r c \varepsilon_0 m_0^2 \omega} \sum_{i,j} \frac{1}{L_T} \int_0^{2\pi} \frac{d\phi}{2\pi} \int_0^{\infty} \frac{k_t dk_t}{2\pi} \left|\langle|\Psi_{i,\boldsymbol{k}_t}|\hat{e}\cdot\hat{\boldsymbol{p}}|\Psi_{j,\boldsymbol{k}_t}\rangle\right|^2 \times \left[f_c^i(\boldsymbol{k}_t) - f_v^j(\boldsymbol{k}_t)\right] \times L\left(\boldsymbol{k}_t, \hbar\omega, \hbar\omega_{ij}\right) \tag{6}$$

where $n_r$ is the refractive index, $c$ the velocity of light, $\varepsilon_0$ is the vacuum permittivity, $p$ is the momentum operator, $\boldsymbol{k}_t$ is the transverse wave vector, $L_T$ is the total thickness of the superlattice (~60 nm), and $\hbar\omega$ and $\hbar\omega_{ij}$ are the photon and peak absorption energies, respectively. A refractive index of $n_r$= 4 was used in the calculations, which is close to the refractive index values of Si and Ge. $f_v^j$ and $f_c^i$ are the Fermi-Dirac distribution for the j^th valence sub-band with energy $E_v^j$ and the i^th conduction sub-band with energy $E_c^i$, respectively. They are given by

$$f_c^i(\boldsymbol{k}_t) = \frac{1}{1 + e^{\frac{E_c^i(\boldsymbol{k}_t) - F_i}{k_B T}}}$$
$$f_v^j(\boldsymbol{k}_t) = \frac{1}{1 + e^{\frac{E_v^j(\boldsymbol{k}_t) - F_j}{k_B T}}} \tag{7}$$

and $F_i, F_j$ are the quasi-Fermi levels. Furthermore, $L$ is the normalized Gaussian function defined as

$$L(k_t, \hbar\omega) = \frac{1}{\gamma\sqrt{2\pi}} \exp\left(-\frac{\left(E_{c,n}(k_t) - E_{v,m}(k_t) - \hbar\omega\right)^2}{2\gamma^2}\right) \tag{8}$$

where $\gamma$ is the linewidth parameter of the interband transitions. A value of 80 meV was used for $\gamma$ in the calculations.

In this work, the studied SLs are intrinsic, therefore the Fermi-level lies in the middle of the effective band gap, and there is no quasi-Fermi-level separation.

In the case of the 14-band $k{\cdot}p$ model, the interaction of the p-type conduction bands with the valence band creates an in-plane anisotropic behavior that prevents the use of the axial approximation. [1] Therefore, this approximation was not used in this work.

**Effect of Interfacial Broadening on Quantum Confinement**

To disentangle the effect of quantum confinement from interfacial broadening, the absorption coefficient of SiGe/Si SL ($m$=3) was evaluated for different well thickness $t$ from 5 to 9 nm and without (Fig. S2a) and with (Fig. S2b) the effect of interfacial broadening.

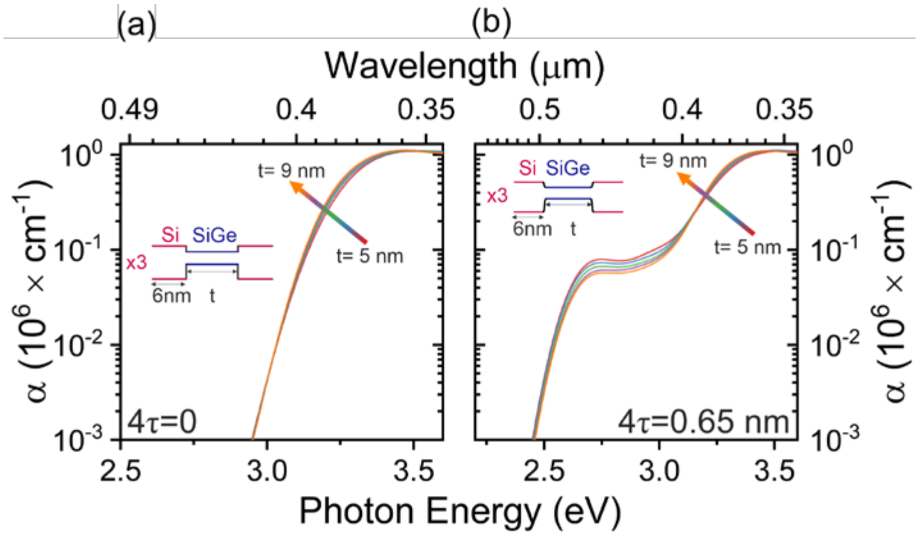


Figure S2: Effect of SiGe well thickness on the absorption coefficient without any interfacial broadening (a) compared to the behavior in presence of interfacial broadening (b).

**Effect of Interfacial Broadening on band structure**

In order to better assess and visualize the effect of the interfacial broadening on the electronic properties of the SiGe/Si SL ($m$=3), Fig. S3 highlights the band structure evaluated with the 14-band $k{\cdot}p$ with (panel a) and without (panel b) interfacial broadening. Clearly, interfacial broadening induces the appearance of an additional band (blue cyan) within the band gap of the heterostructure. This induces a modification in the optical absorption as shown in the main text.

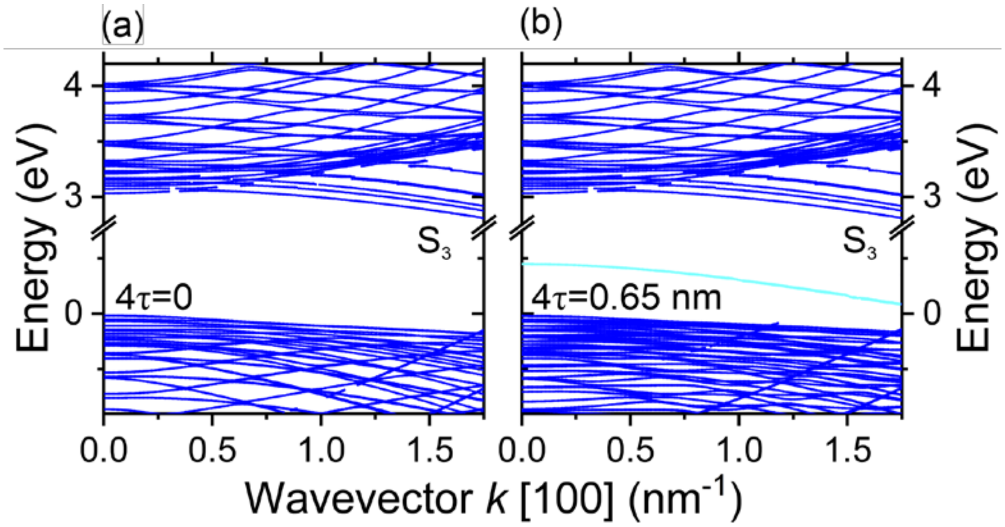


Figure S3: Effect of interfacial broadening on the band structure of the $S_3$ SL evaluated using the 14-band $k{\cdot}p$ with (panel a) and without (panel b) interfacial broadening.

**Inverse Estimation of Smeared Interfaces after Annealing**

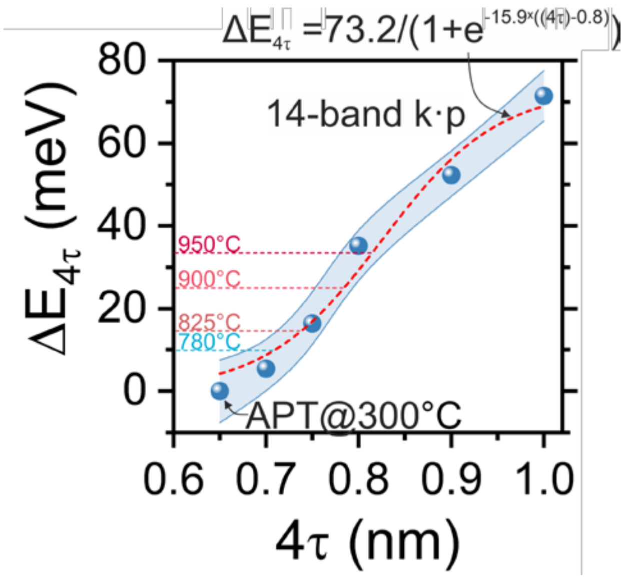


Figure S4: The energy shift $\Delta E_{4\tau}$ of the $S_3$ SL defined as the difference between the experimental $E_{4\tau}$ CP at 4τ = 0.65nm (measured with APT) and the 14-band $k{\cdot}p$ $E_{4\tau}$ CP calculated at different interfacial width (4τ) ($\Delta E_{4\tau} = E_{4\tau=0.65nm} - E_{4\tau}$). The energy shift evolution is fitted to a sigmoid law. Next, the measured experimental shift, associated to a given annealing temperature (Fig.4b) serve to find the corresponding interfacial broadening induced from the annealing process.

## S2. Structural characterization of all SLs

Table 2: Summary of $(Si)_m/(Si_{1-x}Ge_x)_m$ samples measured with AFM, APT, XTEM, HRXRD, and SE in this work.

| Sample No. | Mean $x$ in $Si_{1-x}Ge_x$ [(a)] | Mean period thickness in nm [(a)] from | | | | Total SL thickness (XTEM) (nm) | Mean interfacial broadening $\mathcal{L}$ $(nm)$ |
|---|---|---|---|---|---|---|---|
| | | XTEM | | APT | | | |
| | | $Si_{1-x}Ge_x$ | Si | $Si_{1-x}Ge_x$ | Si | | |
| $S_3$ | 0.293±0.023 | 7.3±0.2 | 6.0±0.2 | 8.3±2.0 | 7.7±0.1 | 40 | 0.65 |
| $S_6$ | 0.295±0.007 | 5.8±0.3 | 4.3±0.2 | 6.4±0.4 | 5.5±0.2 | 61 | 0.70 |
| $S_{12}$ | 0.255±0.003 | 2.6±0.2 | 2.0±0.1 | 2.5±0.3 | 1.6±0.3 | 54 | 1.42[(b)] |
| $S_{16}$ | 0.247±0.040 | 2.2±0.3 | 1.3±0.2 | 2.3±0.4 | 1.3±0.2 | 56 | 0.59 |

(a) The mean includes the last $Si_{1-x}Ge_x$ layer which had grown thicker and with higher Ge content than the remaining $Si_{1-x}Ge_x$ layers. The Ge content in column was estimated from APT measurement and not HRXRD
(b) The interfacial broadening was estimated from EELS and not APT for $S_{12}$.

## S3. Atom Probe Tomography (APT) Characterization

Atom probe tomography (APT) was performed using a UV laser-assisted local electrode atom probe (LEAP 5000). Evaporation of individual atoms was achieved by focusing a UV laser (λ=355nm), with a spot diameter of ∼5 μm and a pulse duration of ∼15 ps. The evaporation rate, the laser pulse repetition-rate, and energy per pulse were 0.5-1.0 ion pulse$^{-1}$, 250-500 kHz, and 3-20 pJ, respectively. The base temperature and base pressure within the APT chamber were 30 K and $2 \times 10^{-11}$ Torr, respectively. The three-dimensional (3D) reconstruction was performed using Cameca's integrated visualization and analysis software (IVAS). The sample preparation for the APT measurements were done in a dual-channel focussed ion-beam (Dual-FIB) microscope, using the standard lamella lift-out and tip sharpening techniques. 2-3 tips from each sample were prepared and analyzed in APT to examine the fidelity of the reconstructions and gain better accuracy by averaging the interfacial widths across different data sets. After reconstruction, atoms located within a cylindrical volume of diameter 30 nm, placed at the centre of the 3D reconstruction around the [001] pole, was extracted and analysed. Next, the heterointerfaces between the Si and the SiGe layers was identified as iso-concentration surfaces, defined at 50% of

the mean Ge concentration of the SiGe layers. Then, the composition of Ge and Si was extracted, as 1D concentration profile (defined at a bin-width of 0.2 nm) from the atoms extracted from within the cylinder of diameter 30 nm at the centre of each data set. A quantitative evaluation of the interdiffusion at the Si/SiGe and SiGe/Si interfaces was performed by fitting the APT Ge compositional profile in Fig. S5a with a superposition of sigmoid profile functions for each interface defined as

$$f(x) = V + \sum_{i=1}^{N} \frac{C_i}{1 + e^{-\frac{(x_i \pm x)}{\tau_i}}} \quad (9)$$

where $V$ is a vertical positioning parameter (equal to 0 for the APT Ge profile, and ≠0 for the EELS Ge profile), and $C$ is a scaling parameter representing the Ge content in the SiGe layer. The sign of x determines if the interface is of Si/SiGe type (positive or increasing Ge content) or of SiGe/Si type (negative or decreasing Ge content). The parameter $\tau$ represent the sharpness of the interface and the interfacial broadening $\mathcal{L}$ is exactly $4\tau$ and represents 10% and 90% of the asymptotic limit value of the maximum Ge content. The result of the sequential least square programming (SLSQP) algorithm is shown in Fig. S5b.

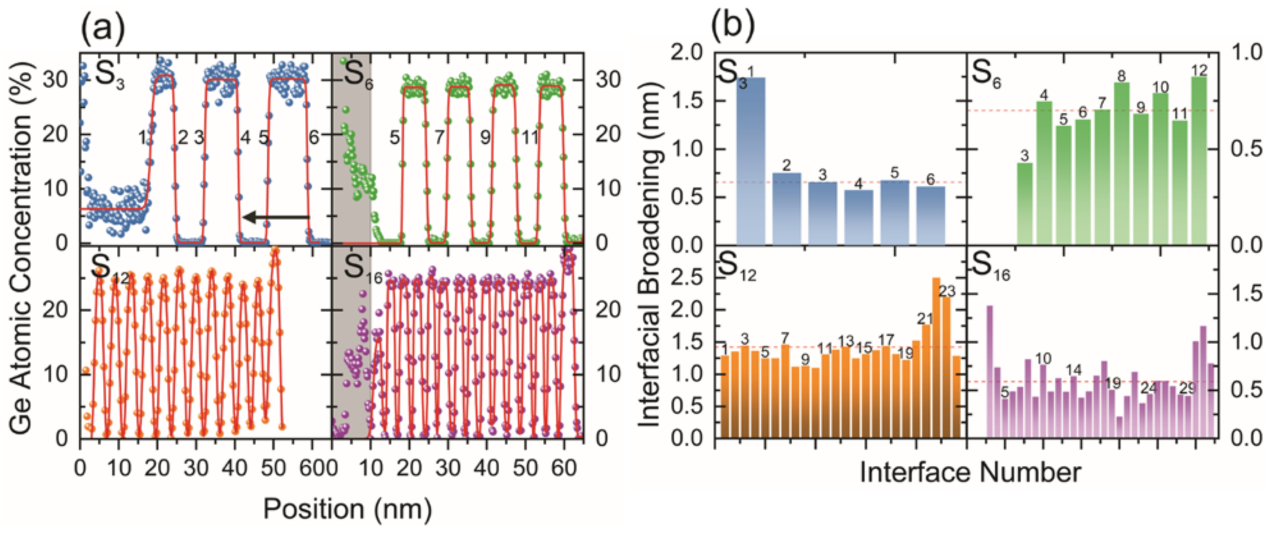


Figure S5: (a) Ge atomic concentration (%) for the 4 SLs estimated with APT for the as-grown $S_3$, $S_6$ and $S_{16}$ SLs and with EELS for the $S_{12}$ SLs. The grey shaded area highlights the region where the tip was damaged during FIB preparation. The odd numbers indicate the Si/SiGe interfaces, and the red curve is the SLSQP fit for the Ge profile following Eq. 9. The black arrow is the growth direction, opposite to the tip evaporation direction. (b) The interfacial broadening for all the SLs at each interface identified in panel a. The dashed red lines are the average interfacial broadening (0.65 nm for $S_3$, 0.7 nm for $S_6$, 1.42 nm for $S_{12}$, and 0.59 nm for $S_{16}$)

## S4. Characterization of lattice Strain

Raman spectroscopy measurements were done using a commercial Renishaw Invia spectrometer using the 514 nm laser line, under ambient conditions. The back-scattered signal was collected using a 20X Olympus objective (NA = 0.75) and diffracted using an 1800 lines/mm grating towards a liquid nitrogen cooled CCD camera. The laser power density was maintained at a nominal value of 0.05 mW/μm$^2$ to minimize any laser induced heating.

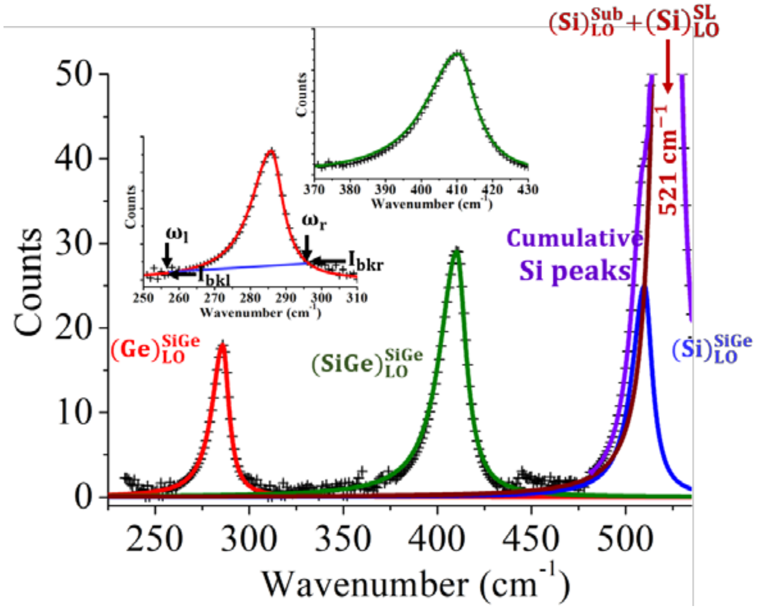


Figure S6: Raman spectra of sample S-6 showing Ge-LO mode of the SL (red), SiGe-LO mode (green) and Si-LO mode. The Si-LO mode consists of the Si-Si mode from the SiGe layer of the SL at 509.9 cm$^{-1}$ (deep blue), as well as that from the Si substrate and the Si layer of the SL at 520.8 cm$^{-1}$ (brown). The cumulative fit of the two Si modes is shown in purple. Inset: The Ge-LO mode and the SiGe-LO modes has been highlighted.

To estimate the residual lattice strain, the Raman peak positions was evaluated in realm of the shift due to the composition as well as due to strain. For this, the Ge-LO mode and the SiGe-LO mode originating from the SiGe layers of the SL were fitted with an exponentially modified Gaussian equation to extract the peak position. The evolution of the LO modes of a $Si_{1-x}Ge_x$ virtual substrate under the influence of both composition (x) and strain (ε) can be written as [26]

$$\omega_{Si-Si} = 520 - 70.5x - 830\varepsilon$$

$$\omega_{Ge-Ge} = 282.5 + 16x - 384\varepsilon$$

$$\omega_{SiGe-SiGe} = 400.5 + 16x - 575\varepsilon$$

The SiGe layers of sample $S_6$ possess a mean Ge composition (x) of 28.5 at.%. The extracted peak positions are 286.07 cm$^{-1}$ for the Ge-LO mode, 409.11 cm$^{-1}$ for the SiGe-LO mode, and 509.96 cm$^{-1}$ for the Si-LO mode from the SL. Since the Si-LO mode from the SL is masked by the stronger peak from the substrate, it was not considered for the analysis. The value of ε was thus estimated from the Ge-LO mode and the SiGe-LO mode. The average (from $\omega_{\mathrm{Ge-Ge}}$ and $\omega_{\mathrm{SiGe-SiGe}}$) was estimated to be 0.00864 or 0.864%. With 28.5 at. % Ge in the SiGe layers, the estimated misfit (f) between Si and the SiGe layers is 0.91% at room temperature. Using the relation $\varepsilon = -\mathrm{f}(1-\mathrm{r})$ the degree of strain relaxation (r) was estimated to be only 5.4$\pm$1%. The uncertainly stems from two sources: the uncertainty in the measured Ge concentration (Δx) as well as the uncertainty in the measured peak position (Δω). The SiGe layers are thus close to being fully strained.

## S5. Atomic Force Microscopy (AFM) Characterization

In the 20 µm ×20 µm AFM map of the as-grown $S_3$ and the 10 µm ×10 µm AFM maps for the as-grown $S_6$, $S_{12}$ and $S_{16}$ SLs shown in Fig. S7, a root mean square (RMS) value of 0.44 nm, 0.53 nm, 0.55 nm and 0.64 nm is estimated respectively for the sample surface. While constructing the SE optical model, a surface layer was considered to mimic the AFM measured surface roughness and was modeled with the Bruggeman effective medium approximation (BEMA). The thickness of the BEMA layer was fixed to that of the RMS extracted from the AFM characterization.

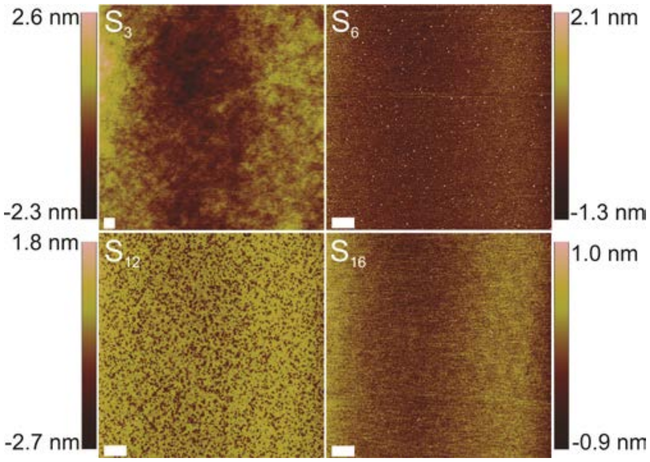


Figure. S7: AFM maps for the as-grown $S_3$ (20 µm× 20µm map), $S_6$, $S_{12}$ and $S_{16}$ SLs extracted from a 10 µm× 10µm AFM maps. Scale bar is 1 µm in all maps.

## S6. Spectroscopic Ellipsometry (SE)

The variable angle spectroscopic ellipsometry (VASE) uses change in the state of polarization of light upon reflection for characterization of surfaces, interfaces, and thin films. SE measurement in $Si_{1-x}Ge_x$/Si heterostructures multilayer systems can enable the assessment of the critical point (CP) energies as well as information on thickness, crystallinity, roughness, and composition of individual layers. The complex pseudo-dielectric function $\langle\varepsilon(\omega)\rangle = \langle\varepsilon_1(\omega)\rangle + i\langle\varepsilon_2(\omega)\rangle$ can be derived from SE data by using a two-phase model, and is defined as follows

$$\varepsilon(\omega) = \sin^2\varphi + \sin^2\varphi\tan^2\varphi\left[\frac{1-\rho}{1+\rho}\right]^2 \qquad (10)$$

where $\varphi$ is the angle of incidence (AOI). For each sample, the SE measurements were undertaken for energy ranging between 0.5 eV and 6 eV with a step size of 0.01 eV at several AOI (between 60° and 80° with a 5° step) to increase the accuracy of the subsequent analysis. The non-focused spot size has a diameter of around 2 mm, and so a projected major axis between 4.7 and 7.7 mm (for angles of 65° and 75°, respectively). Fig. S8a present the ellipsometric parameters Ψ and Δ for the $S_3$ SL, whereas Fig. S8b show the same parameters for the $S_{16}$ SL. Besides, the "point-by-point" optical model is superimposed with the experimental data set to validate the quality of the built optical model. Once the model has been built, one varies the physical parameters using the Levenberg-Marquardt algorithm to minimize the mean-squared error (MSE). The MSE is a figure of merit for how well the present set of parameters fits the ellipsometric data. For sample $S_3$ and $S_{16}$, the MSE was estimated to be 0.892 and 0.942, respectively, which is an indication of the excellent optical model. A multilayer optical model including ($SiO_2$/SL/Si) structure was used for accurate treatment of the experimental data. The WVASE© software library provides the optical constants of the $SiO_2$ native oxide layers, [27] whereas the double-side polished Si substrate was measured independently and the Johs-Herzinger (J-H) model was considered to extract the Si dielectric function. [28] The optical properties of the superlattice are fit to different optical models. Three different models were considered. The first is based upon the parametric semiconductor (PSEMI) model developed by J-H. [28] The second is a simple Gaussian oscillator (not shown in Fig. S9) and the third is a "point-by-point" (also known as "wavelength-by-wavelength") model.

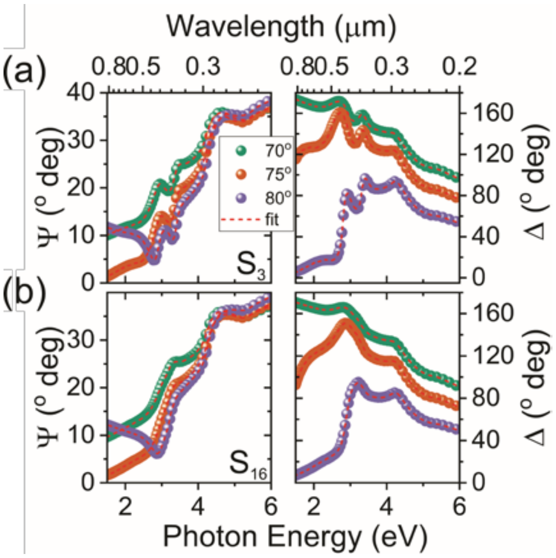


Figure S8: Spectroscopic ellipsometry parameters Ψ and Δ for (a) $S_3$ and (b) $S_{16}$ SLs, at different AOI. The red line represents the fit to the experimental measurement deduced from the point-by-point optical model, elaborated previously in details.

The point-by-point optical model generates a pair of raw optical constants for each measured wavelength. The benefit of using a "point-by-point" approach is that it leads to the actual measured optical constants unaltered by any particular *a priori* model assumption, fitting or smoothing such is the case when a general oscillator model is used. Kramers-Kronig consistency was verified by comparing the "point-by-point" fit result to the oscillator-based fit as shown in Fig. S9. Fig. S9 presents the fit results with (green full line and purple-dashed line) and without (blue line) an additional oscillator below 3 eV. The added oscillator accounts for the broad peak observed below 3 eV (see the enlarged log-log plot in Fig. S9). Above 3 eV, the PSEMI oscillator model was assumed and unaltered for each of the critical points around 3 eV, 3.5eV, 4.1eV and 5.3eV. Below 3eV, the 3 previous models were considered to determine the most suitable one. In the one hand, if no additional oscillator is considered below 3 eV, then the mean residual is equal to 14.7%. On the other hand, a noticeable reduction in the mean residual is obtained when an oscillator is considered. For instance, the gaussian oscillator leads to a mean residual of 3.8%. The mean residual of the PSEMI is reduced to 1.8% and that of the point-by-point models to 0.4%. The PSEMI model is plagued with oscillations that arise from the different numerical components of the oscillator, whereas the point-by-point model shows a near-to zero residual, confirming the reliability of this approach.

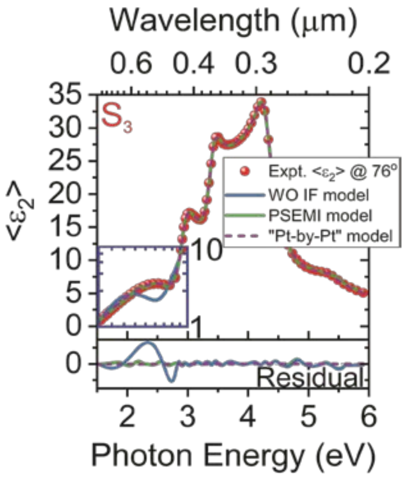


Figure S9: Experimental pseudo-dielectric function of the S3 SL acquired at 76°. The blue line is the fitted model without accounting for the additional transition below 3 eV, whereas the green and purple-dashed lines are the fit results when considering an additional PSEMI oscillator and the point-by-point model, respectively. The blue log-log plot is an enlarged region to better assess the need for an additional oscillator to fit the experimental results.

## S7. Fitting second derivative lineshapes

The point-by-point dielectric function for the superlattice was smoothed using the Savitzky-Golay (SG) routine in the MATLAB® software using the "*sgolayfilt*" routine. The raw and smoothed data were compared very closely throughout the energy range to ensure that the smoothing process was sufficiently minimizing noise without affecting spectral features. It is critical to avoid over-smoothing the data; otherwise, subtle features such as peak broadening could be lost. Optimal smoothing was achieved with a fifth polynomial order and a window of 15 data points. Next, the second derivative of the dielectric function was fit to the following lineshape

$$\frac{d^2\varepsilon}{d\omega^2} = \begin{cases} n(n-1)Ae^{i\phi}\left(\omega - E_j + i\Gamma\right)^{n-2}, & n \neq 0 \\ Ae^{i\phi}\left(\omega - E_j + i\Gamma\right)^{-2}, & n = 0 \end{cases} \tag{11}$$

where $E_j$ is the threshold energy, $\Gamma$ is the broadening, and $A$ is a measure of the strength of the CP, while $\phi$ represents the amount of mixture of adjacent CP's due to excitonic effects. The exponent $n$ equals -0.5, 0, 0.5, or -1 for one dimensional (1D), 2D, 3D, or exitonic interactions, respectively. Data fits were performed simultaneously for the real and imaginary parts of $d^2\varepsilon/d\omega^2$ using a global optimization procedure based on the differential evolution (DE) algorithm. [29] To iteratively fit and extract the critical point parameters from the second derivative of the dielectric constant, a robust numerical approach is used to permit an automatic, and accurate estimation of the CP parameters. To this end, differential evolution (DE) was used to fit the theoretical line-

shapes to the second derivative of the dielectric function. The use of global optimization approach in the context of line-shape fitting is justified by the fact that the objective function is non-linear, noisy, and has many local minima, rendering the possibility to solve such problems analytically difficult. Thus, DE can be used to find approximate solutions to such problems. Nevertheless, the choice of the objective function to optimize constitutes an important step of the fitting process. *De facto*, the objective function for model parameter determination should be chosen in such a manner that discrepancies between the experimental and calculated values for both parts of the index of refraction (real and imaginary) are minimized simultaneously. Consequently, the objective function in this work is defined as follows: [30]

$$F = \sum_{i=1}^{N} \left[ \left| \frac{\varepsilon_1(\omega_i)}{\varepsilon_1^{expt}(\omega_i)} - 1 \right| + \left| \frac{\varepsilon_2(\omega_i)}{\varepsilon_2^{expt}(\omega_i)} - 1 \right| \right]^2 \quad (12)$$

where the summation is performed over $N$ available experimental points, while $\varepsilon_1^{expt}(\omega_i)$, $\varepsilon_1(\omega_i)$ and $\varepsilon_2^{expt}(\omega_i)$, $\varepsilon_2(\omega_i)$ refer to the experimental and calculated values of the real and imaginary parts of the dielectric constant at point $\omega_i$. Also, the expressions $\varepsilon_2(\omega_i) - \varepsilon_2^{expt}(\omega_i)$ were considered instead of $\varepsilon_2(\omega_i)/\varepsilon_1^{expt}(\omega_i) - 1$ for $\varepsilon_1^{expt}(\omega_i) = 0$. The objective function $F$ considers cross-correlation terms for the real and imaginary parts of the dielectric constant. These cross-correlation terms ensure that the solution gives an equal quality fit for both the real and imaginary parts of the dielectric constant. The algorithm starts from arbitrary initial parameters and high objective function values, and in the final phase it has difficulties in distinguishing among minima with similar objective function values, which can be quite distant in the model parameter space. When this happens, the following process was employed; the imaginary part (or the real part) was to be fitted first, and the best-fit parameters obtained from that fit were used as the starting iterations for the fit to the real part (or imaginary part), and this is repeated iteratively until the difference between the fitted and experimental data is smaller than a convergence criteria set by the user (around $10^{-3}$). The full result of the fitting process is shown in Table S2, where the lineshape parameters as well as the coefficient of determination are presented.

Table S2: Room-temperature interband critical-point best-fit parameters for all the studied superlattices. The accuracy of the fits to the real and imaginary second-derivative spectra for most parameters is quantified through the coefficient of determination $R^2$.

| **Sample** | **R²** | **Assignment** | **RTSE** | | | | | |
|---|---|---|---|---|---|---|---|---|
| | | | *A* | $E_i$ *(eV)* | $\Gamma$ *(meV)* | $\phi$*(deg)* | $n$ | Type |
| $S_3$ | 0.994 | $\boldsymbol{E_{4\tau}}$ | **8.5213** | **2.1212** | **42.95** | **130** | **0.43** | (3D) |
| | 0.999 | $E_1^a$ | 1.7052 | 2.9249 | 109.88 | 7 | -0.95 | excitonic |
| | 0.994 | $E'_0$ | 49.2314 | 3.2110 | 80.68 | 43 | 0.5 | (3D) |
| | 0.996 | $E_1^b$ | 1.6542 | 3.4134 | 129.72 | 65 | -1 | excitonic |
| $S_6$ | 0.978 | $\boldsymbol{E_{4\tau}}$ | **75.3927** | **2.1995** | **82.76** | **173** | **0.23** | (3D) |
| | 0.975 | $E_1^a$ | 1.64 | 2.9334 | 112.25 | 133 | -1 | excitonic |
| | 0.992 | $E'_0$ | 4.5485 | 3.2224 | 250.43 | 79 | -1 | excitonic |
| $S_{12}$ | 0.945 | $\boldsymbol{E_{4\tau}}$ | **7.1092** | **2.1987** | **44.38** | **136** | **0.45** | (3D) |
| | 0.981 | $E_1^a$ | 25.6083 | 2.9530 | 73.47 | 83 | 0.5 | (1D) |
| | 0.989 | $E'_0$ | 2.8536 | 3.2194 | 210.35 | 60 | -1 | excitonic |
| $S_{16}$ | 0.988 | $\boldsymbol{E_{4\tau}}$ | **113.877** | **2.0951** | **59.19** | **140** | **0.48** | (3D) |
| | 0.978 | $E'_0$ | 293.288 | 2.9918 | 109.35 | -28 | 0 | (2D) |
| | 0.984 | $E_1^b$ | 3.4869 | 3.2141 | 221.19 | 13 | -1 | excitonic |

## References


[1] M. El kurdi, G. Fishman, S. Sauvage, and P. Boucaud, *Comparison between 6-Band and 14-Band K·p Formalisms in SiGe/Si Heterostructures*, Phys. Rev. B - Condens. Matter Mater. Phys. **68**, 165333 (2003).

[2] T. B. Bahder, *Eight-Band k · p Model of Strained Zinc-Blende Crystals*, Phys. Rev. B **41**, 11992 (1990).

[3] N. A. Čukarić, M. Ž. Tadić, B. Partoens, and F. M. Peeters, *30-Band K·p Model of Electron and Hole States in Silicon Quantum Wells*, Phys. Rev. B **88**, 205306 (2013).

[4] D. Rideau, M. Feraille, L. Ciampolini, M. Minondo, C. Tavernier, H. Jaouen, and A. Ghetti, *Strained Si, Ge, and Si1-x Gex Alloys Modeled with a First-Principles- Optimized Full-Zone Kp Method*, Phys. Rev. B - Condens. Matter Mater. Phys. **74**, 195208 (2006).

[5] R. R. Reeber and K. Wang, *Thermal Expansion and Lattice Parameters of Group IV Semiconductors*, Mater. Chem. Phys. **46**, 259 (1996).

[6] B. A. Foreman, *Elimination of Spurious Solutions from Eight-Band K· p Theory*, Phys. Rev. B **56**, R12748 (1997).

[7] S. Ridene, K. Boujdaria, H. Bouchriha, and G. Fishman, *Infrared Absorption in Si/Si1-XGex/Si Quantum Wells*, Phys. Rev. B - Condens. Matter Mater. Phys. **64**, 853291 (2001).

[8] J. P. Dismukes, L. Ekstrom, and R. J. Paff, *Lattice Parameter and Density in Germanium-Silicon Alloys 1*, J. Phys. Chem. **68**, 3021 (1964).

[9] D. J. Paul, *8-Band K·p Modelling of Mid-Infrared Intersubband Absorption in Ge Quantum Wells*, J. Appl. Phys. **120**, 043103 (2016).

[10] O. Madelung, U. Rössler, and M. Schulz, *Group IV Elements, IV-IV and III-V Compounds. Part b - Electronic, Transport, Optical and Other Properties*, Vol. b (Springer-Verlag, Berlin/Heidelberg, 2002).

[11] Y. P. Varshni, *Temperature Dependence of the Energy Gap in Semiconductors*, Physica **34**, 149 (1967).

[12] C. G. Van de Walle, *Band Lineups and Deformation Potentials in the Model-Solid Theory*, Phys. Rev. B **39**, 1871 (1989).

[13] H. J. McSkimin, *Measurement of Elastic Constants at Low Temperatures by Means of Ultrasonic*

*Waves–Data for Silicon and Germanium Single Crystals, and for Fused Silica*, J. Appl. Phys. **24**, 988 (1953).

[14] L. D. Laude, F. H. Pollak, and M. Cardona, *Effects of Uniaxial Stress on the Indirect Exciton Spectrum of Silicon*, Phys. Rev. B **3**, 2623 (1971).

[15] M. Chandrasekhar and F. H. Pollak, *Effects of Uniaxial Stress on the Electroreflectance Spectrum of Ge and GaAs*, Phys. Rev. B **15**, 2127 (1977).

[16] L. Viña, S. Logothetidis, and M. Cardona, *Temperature Dependence of the Dielectric Function of Germanium*, Phys. Rev. B **30**, 1979 (1984).

[17] P. Lautenschlager, M. Garriga, L. Vina, and M. Cardona, *Temperature Dependence of the Dielectric Function and Interband Critical Points in Silicon*, Phys. Rev. B **36**, 4821 (1987).

[18] C. G. Van de Walle and R. M. Martin, *Theoretical Calculations of Heterojunction Discontinuities in the Si/Ge System*, Phys. Rev. B **34**, 5621 (1986).

[19] I. Balslev, *Influence of Uniaxial Stress on the Indirect Absorption Edge in Silicon and Germanium*, Phys. Rev. **143**, 636 (1966).

[20] J. Weber and M. I. Alonso, *Near-Band-Gap Photoluminescence of Si-Ge Alloys*, Phys. Rev. B **40**, 5683 (1989).

[21] D. De Salvador, M. Petrovich, M. Berti, F. Romanato, E. Napolitani, A. Drigo, J. Stangl, S. Zerlauth, M. Mühlberger, F. Schäffler, G. Bauer, and P. Kelires, *Lattice Parameter of Alloys*, Phys. Rev. B - Condens. Matter Mater. Phys. **61**, 13005 (2000).

[22] B. A. Foreman, *Analytical Envelope-Function Theory of Interface Band Mixing*, Phys. Rev. Lett. **81**, 425 (1998).

[23] E. Ivchenko, A. Y. Kaminski, and U. Rössler, *Heavy-Light Hole Mixing at Zinc-Blende (001) Interfaces under Normal Incidence*, Phys. Rev. B - Condens. Matter Mater. Phys. **54**, 5852 (1996).

[24] F. Szmulowicz, H. Haugan, and G. J. Brown, *Effect of Interfaces and the Spin-Orbit Band on the Band Gaps of InAs/GaSb Superlattices beyond the Standard Envelope-Function Approximation*, Phys. Rev. B **69**, 155321 (2004).

[25] P.-F. Qiao, S. Mou, and S. L. Chuang, *Electronic Band Structures and Optical Properties of Type-II Superlattice Photodetectors with Interfacial Effect*, Opt. Express **20**, 2319 (2012).

[26] J. C. Tsang, P. M. Mooney, F. Dacol, and J. O. Chu, *Measurements of Alloy Composition and*

*Strain in Thin GexSi1-x Layers*, J. Appl. Phys. **75**, 8098 (1994).

[27] E. D. Palik, *Handbook of Optical Constants of Solids* (Academic Press, London, UK, 1998).

[28] C. M. Herzinger, B. Johs, W. A. McGahan, J. A. Woollam, and W. Paulson, *Ellipsometric Determination of Optical Constants for Silicon and Thermally Grown Silicon Dioxide via a Multi-Sample, Multi-Wavelength, Multi-Angle Investigation*, J. Appl. Phys. **83**, 3323 (1998).

[29] R. Storn and K. Price, *Differential Evolution – A Simple and Efficient Heuristic for Global Optimization over Continuous Spaces*, J. Glob. Optim. **11**, 341 (1997).

[30] A. B. Djurišić, T. Fritz, and K. Leo, *Modelling the Optical Constants of Organic Thin Films: Impact of the Choice of Objective Function*, J. Opt. A Pure Appl. Opt. **2**, 458 (2000).
